# Supplementary material for: ResNeSt: Split-Attention Networks
Source: arXiv:2004.08955 source file (2020-12-30)
Supplement: Supplementary file 1 [file supp.tex]

% updated April 2002 by Antje Endemann
% Based on CVPR 07 and LNCS, with modifications by DAF, AZ and elle, 2008 and AA, 2010, and CC, 2011; TT, 2014; AAS, 2016; AAS, 2020

\documentclass[review]{cvpr}

\usepackage{times}
\usepackage{epsfig}
\usepackage{amsmath,amssymb} % define this before the line numbering.
\usepackage{color}
\usepackage{cite}
\usepackage{epsfig}
\usepackage{graphicx}
\usepackage{subfig}

\usepackage{cite}
\usepackage{comment}
\usepackage{adjustbox}
\usepackage{textcomp}
\usepackage{array,multirow,graphicx}
\usepackage[table]{xcolor}
\usepackage{colortbl}
\usepackage{bbm}
\usepackage{makecell}
\usepackage[percent]{overpic}

\usepackage{booktabs}
\usepackage{arydshln}
\usepackage{url}

\usepackage{pgfplots}
\usepackage{filecontents}
\usepackage{wrapfig}

\usepackage{tikz}
\usetikzlibrary{arrows}
\usetikzlibrary{calc} 
\usepackage{placeins}

\usepackage{lipsum}

% Include other packages here, before hyperref.

% If you comment hyperref and then uncomment it, you should delete
% egpaper.aux before re-running latex.  (Or just hit 'q' on the first latex
% run, let it finish, and you should be clear).
\usepackage[pagebackref=true,breaklinks=true,colorlinks,bookmarks=false]{hyperref}

\def\best{\bf \cellcolor[gray]{0.85}}
\def\secbest{\cellcolor[gray]{0.92}}

\definecolor{TableRed}{HTML}{800000}
\newcommand{\TextRed}[1]{\textcolor{TableRed}{#1}}

 % *** Enter the CVPR Paper ID here

%\setcounter{page}{4321} % For final version only

\begin{document}

%%%%%%%%% TITLE
\title{Supplementary Material for ResNeSt: Split-Attention Networks}

\author{First Author\\
Institution1\\
Institution1 address\\
{\tt\small firstauthor@i1.org}
\and
Second Author\\
Institution2\\
First line of institution2 address\\
{\tt\small secondauthor@i2.org}
}

\maketitle

\section{Additional Experiments}

% In this section, we include the extra experimental results using ResNeSt. 

\subsection{Comparing to Other ResNet Variants}
For fair comparison, we retrain the proposed ResNeSt and other ResNet variants in the same training recipe. 
In this benchmark, we use a simple training setting to reduce the training cost. 
All the networks are trained for 120 epochs, with a mini-batch of 512. We use 0.2 as the initial learning rate and apply a cosine learning rate decay. 
Standard data augmentation is used including random size crop, horizontal flip, color and lightning jittering. The weight decay is set to 0.0001 and the momentum is 0.9. No other training enhancement or regularization is used in this benchmark. 

\begin{table}
	\small
	\centering
	\renewcommand\arraystretch{1.1}
	\newcommand{\tabincell}[2]{\begin{tabular}{@{}#1@{}}#2\end{tabular}}
	\resizebox{\linewidth}{!}{
		\begin{tabular}{l|c|c|c}
			\toprule[1pt]
			& \#P   &GFLOPs
			&Acc (\%) \\   
% 			\\
% 			\cline{4-5}
% 			&&&224$\times$\\
			\hline
            %\cline{1-5}
			ResNet-50~\cite{he2015deep} & 25.5M & 4.14 & 76.48 \\
			ResNeXt-50~\cite{xie2016aggregated} & 25.0M & 4.24  & 78.17 \\
			%SENet-50 \cite{hu2017squeeze} & {27.7}M & 4.25 & 78.88  \\
			ResNetD-50~\cite{he2019bag} & 25.6M & 4.34 & 76.69 \\
			SKNet-50 \cite{sknet} & 27.5M  & {4.47} & \secbest 78.03  \\
			ResNeSt-50-fast*(\TextRed{\small ours}) & 27.5M & 4.34 & \best 78.73 \\
			\bottomrule[1pt]
		\end{tabular}
	}
	\vspace{1em}
	\caption{Image classification results on ImageNet, comparing our proposed ResNeSt with other ResNet variants of similar complexity in 50-layer configurations. We report top-1 accuracy using crop size of $224$. (* We use ResNeSt-50-fast with 2s8x14d in this benchmark. )
	}
	\label{tab:res_sota}
	%\vspace{-2em}
\end{table}

\input{eccv2020kit/appendix}

%\bibliographystyle{splncs04}
%\bibliography{egbib}

%\clearpage
\FloatBarrier

{\small
\bibliographystyle{ieee_fullname}
\bibliography{egbib}
}

\end{document}
